# Supplementary material for: Field-induced polarisation of Dirac valleys in bismuth
Source: arXiv:1109.2774 source file (2011-09-13)
Supplement: Supplementary file 1 [file Supplementary_material_rs.pdf]

Supplementary material for:

# Field-induced polarisation of Dirac valleys in bismuth

**Methods :** Angular-dependent resistivity was measured both with a PPMS and with a home-made set-up using a piezoelectric rotator to rotate the sample and a pair of Hall sensors to determine the angle. Both yielded similar results. Bismuth single crystals used in this study had a typical size of 1-2 X 1-2 X 4-5 $mm^3$ and a “Residual Resistivity Ratio” (RRR= R(300K)/R(4.2 K)) in the range of 150 to 170. They were characterized as detailed below.

## 1. The temperature dependence of the zero-field resistivity

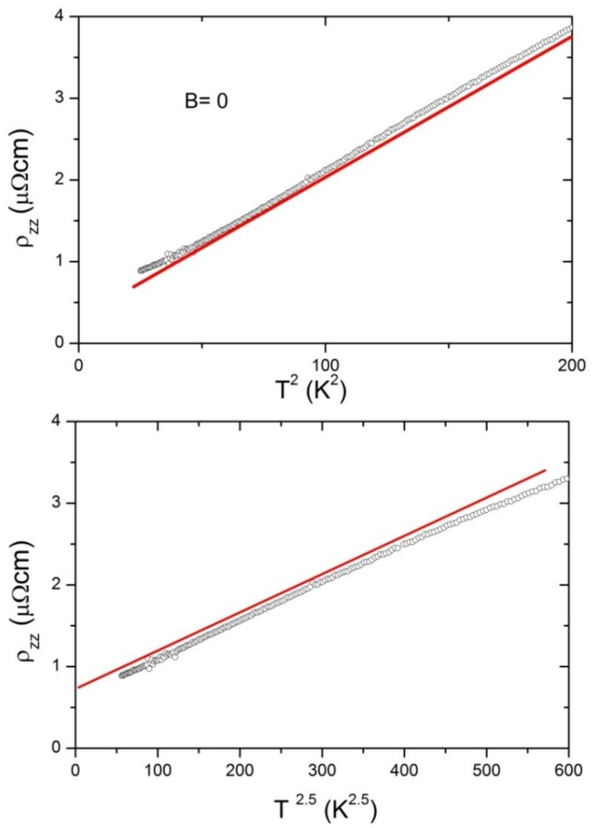


**Fig. S1- Top:** Out-of-plane resistivity (i.e. for a current applied the trigonal axis) as a function of $T^2$ in a bismuth single crystal used in this study. The slope of the red solid line, a guide for eyes, is 12 nΩcm $K^{-2}$. **Bottom:** Same data plotted as a function of $T^{2.5}$.

The resistivity of the sample used to obtain the data of figures 1 and 2 is 0.9 μΩcm at 4.2 K. Give the extremely low carrier density in bismuth ($n_e$=$n_h$ = 3 $10^{17}$ $cm^{-3}$ [S1]), such a conductivity implies an average carrier mobility as large as <μ> ≅1.1 $10^7$ $cm^2V^{-1}$ $s^{-1}$. This average mobility corresponds to an average mean-free-path of about 0.1 mm.

The temperature dependence of the resistivity is shown in Fig.S1 and is close to $T^2$. The slope of this quadratic temperature dependence (12 nΩcm $K^{-2}$ ) is close to what was found in previous studies[S2-S3]. A deviation from the $T^2$ dependence is, however, detectable at low temperature. As seen in the bottom panel of the figure an exponent somewhat larger than 2 yields a better fit to the data.

The origin of inelastic scattering in bismuth has been a subject of controversy and both electron-electron scattering [S2] and phonon-electron [S4] scattering have been put forward. Conventional

phonon scattering is expected to yield a $T^5$ temperature dependence in temperatures below $\Theta_D/5$ ($\Theta_D$=120 K is the Debye temperature [S5]). This is not the case of bismuth, where the exponent of the power law remains close to 2 down to 0.1 K [S3]. The deviation from $T^2$ dependence in bismuth is yet to be understood given the fact that in semi-metallic graphite resistivity unambiguously displays a $T^2$ behavior[S6].

## 2. Low field-magnetoresistance

In bismuth, the weak-field regime ($\omega_c \tau < 1$) characterized by a $B^2$ magnetoresistance is restricted to very low fields[S3,S7]. Fig. S2 shows the low-field resistivity data on one of our samples. At T= 4.2 K, the $B^2$ behavior is detectable at very low fields (B < 0.4 mT).

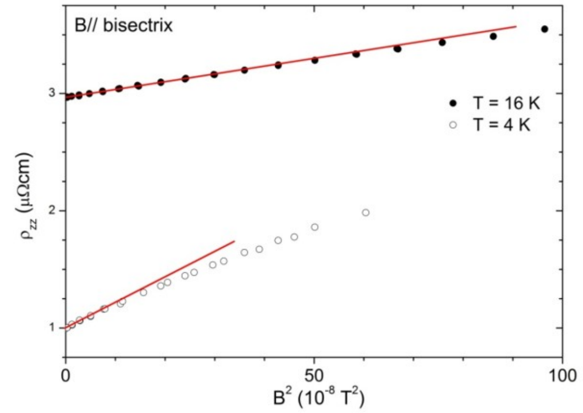


**Fig. S2-** Low-field resistivity of another bismuth single crystal along the trigonal axis as a function of the square of the magnetic field.

The magnitude of the $B^2$ term and the range of validity both scale with mobility. As expected, the mobility lowers at higher temperatures and as a consequence the slope decreases and the range of validity of the quadratic field dependence expands. At 4.2 K, the magnitude of $B^2$ term (0.022 $\Omega$m $T^{-2}$) yields an average mobility of 0.7 $10^7$ $cm^2V^{-1}$ $s^{-1}$ comparable to the one estimated from the absolute magnitude of the resistivity.

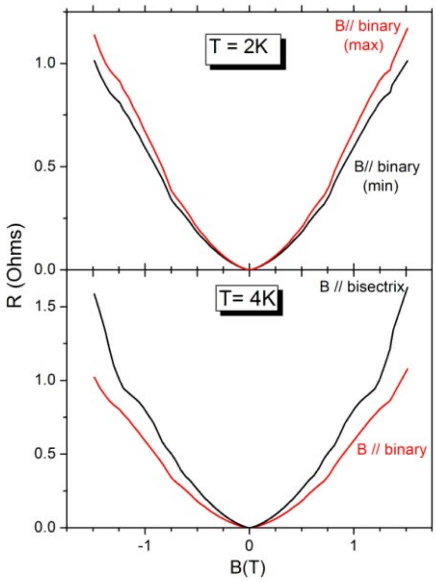


**FIG. S3 Top :** Magnetoresistance when the magnetic field is oriented along two nominally equivalent binary axes. **Bottom :** Magnetoresistance when the magnetic field is oriented along a bisectrix and a binary axis. Quantum oscillations are visible on top of a monotonous background. They represent a modest change overall resistive response. The orientation of magnetic field has a drastic effect on the magnitude of the background.

## 3. Angular magnetoresistance and quantum oscillations

At low temperatures, we can resolve the quantum oscillations of the resistivity (the Shubnikov-de Haas effect). These oscillations are intimately linked to the topology of the pockets of the Fermi surface and their periodicity is affected by the orientation of the magnetic field. However, the angle-dependent magnetoresistance we study here is about the dependence of the non-oscillating back ground on the orientation of the magnetic field. This can be seen in Fig. S3. Both the bisectrix-binary anisotropy and the binary-binary anisotropy (i.e. the loss of the threefold symmetry at high fields and/or low temperatures) are associated with a drastic variation of the background resistive response and not with the amplitude of the quantum oscillations.

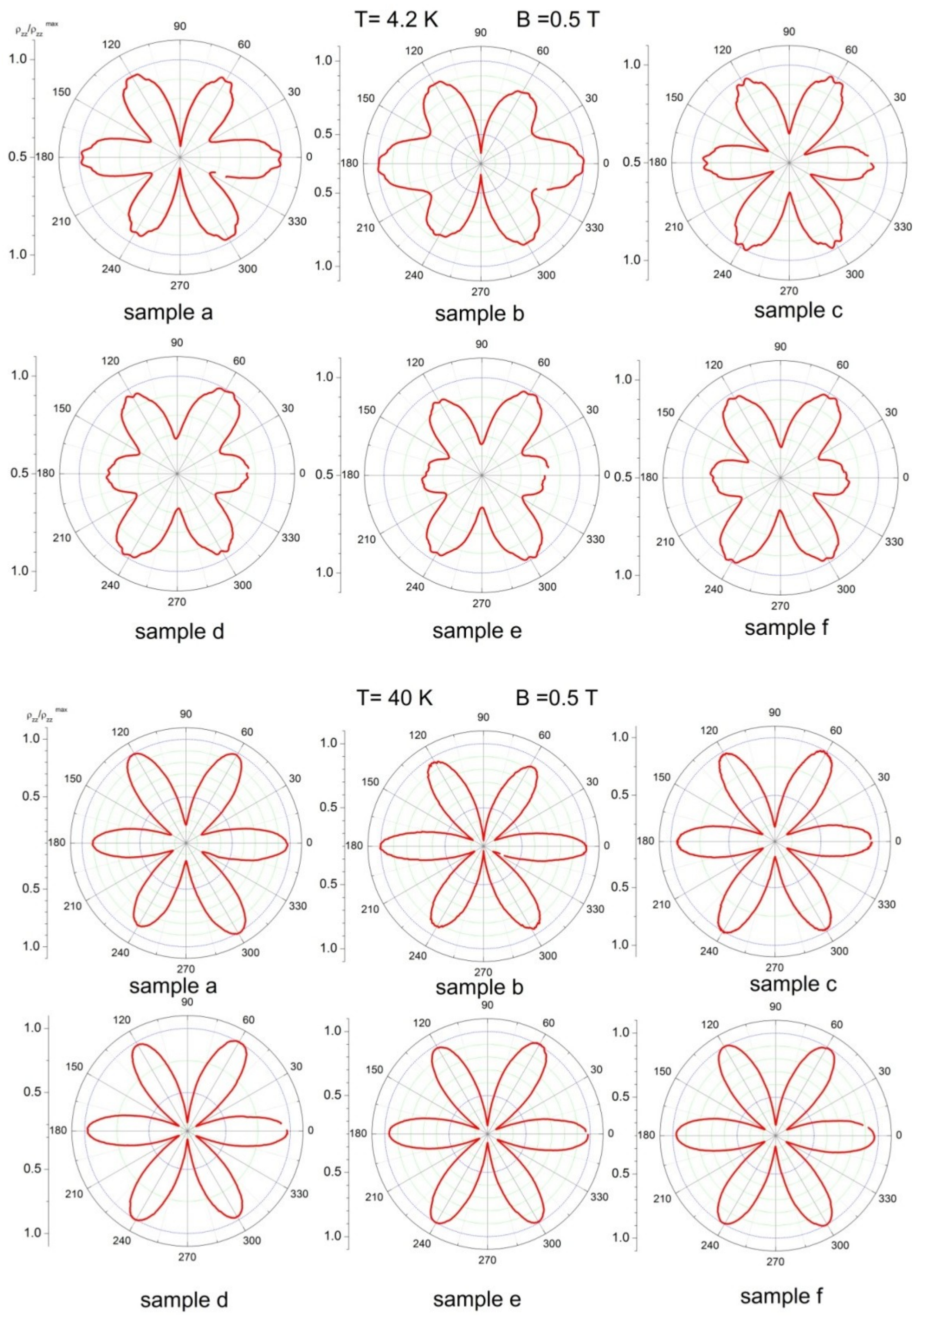


**FIG. S4 Top:** Angular-dependent resistivity in six different single crystals of bismuth at low temperatures. In all samples, the threefold symmetry of the lattice is lost at low temperatures. **Bottom:** Same at 40K. In all samples, the threefold symmetry is recovered, within experimental margin.

## 4. Loss of threefold symmetry in different samples

We studied six different bismuth samples cut from two larger single crystals. As seen in the top panel of Fig. S4, all crystals showed a departure from threefold symmetry, significantly larger than our experimental margin of error. The latter can be seen in the bottom panel, which shows the data for the same samples at 40 K. Samples a, b and c were cut from one large single crystal and samples e, f and g were cut from another large single crystal, with comparable residual resistivities. As seen in the figure, the low-temperature patterns of anisotropy differ in the two single crystals, but are similar in samples cut from the same single crystals. We found that the anisotropic patterns are robust and do not display any significant evolution with thermal recycling. Samples d and e were used for extensive measurements of field dependence.

## 5. Loss of threefold symmetry in field scans

Fig. S5 presents the ratio of magnetoresistance along two interchangeable bisectrix axes as a function of magnetic field at different temperatures in one of the crystals. As seen in the figure, at low temperatures, a difference appears and gradually grows with increasing magnetic field. No sharp anomaly is visible. However, as the temperature is decreased, the transition becomes sharper and one can clearly define a field above which the anisotropy (which was found to be between 7 and 15 percent in different samples) ceases to increase further.

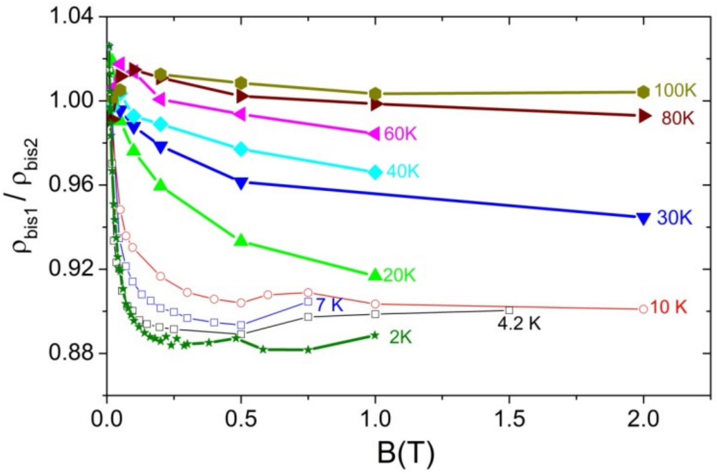


**FIG. S5** The evolution of the ratio of resisitivities for field oriented along two distinct bisectrix axes with temperature. At low temperature the ratio saturates above a threshold magnetic field.

## 6. The origin of empirical fit and its limit of applicability

We analyzed the experimental data by a fit to equation 2. According to this equation, the contribution of each electron valley to the total conductivity has the same angular dependence rotated by $2\pi/3$ radian. For each valley, the angular dependence is:

$$\sigma^{e}_{zz} = \sigma_{bin} / (1+ r \cos^2\phi)$$

This empirical fit is inspired by the well-known semi-classical expression for magnetoconductivity:

$$\sigma(B) = \sigma_0 / [1+ (\omega_c\tau)^2]$$

The angular dependence of magnetoconductivity is set by the angular dependence of the cyclotron frequency (governed by the anisotropy of the cyclotron mass) and the scattering time. The cyclotron mass is largest when the field is parallel to the binary axis and lowest when the field is parallel to the bisectrix axis. As a consequence, the magnetoconductivity is largest (i.e. the magnetoresistivity is lowest) when the field is parallel to the binary axis and is lowest when the field is parallel to the bisectrix axis. As seen in Fig. S6, this empirical fit is quite successful at high temperatures, but fails when the threefold symmetry is lost.

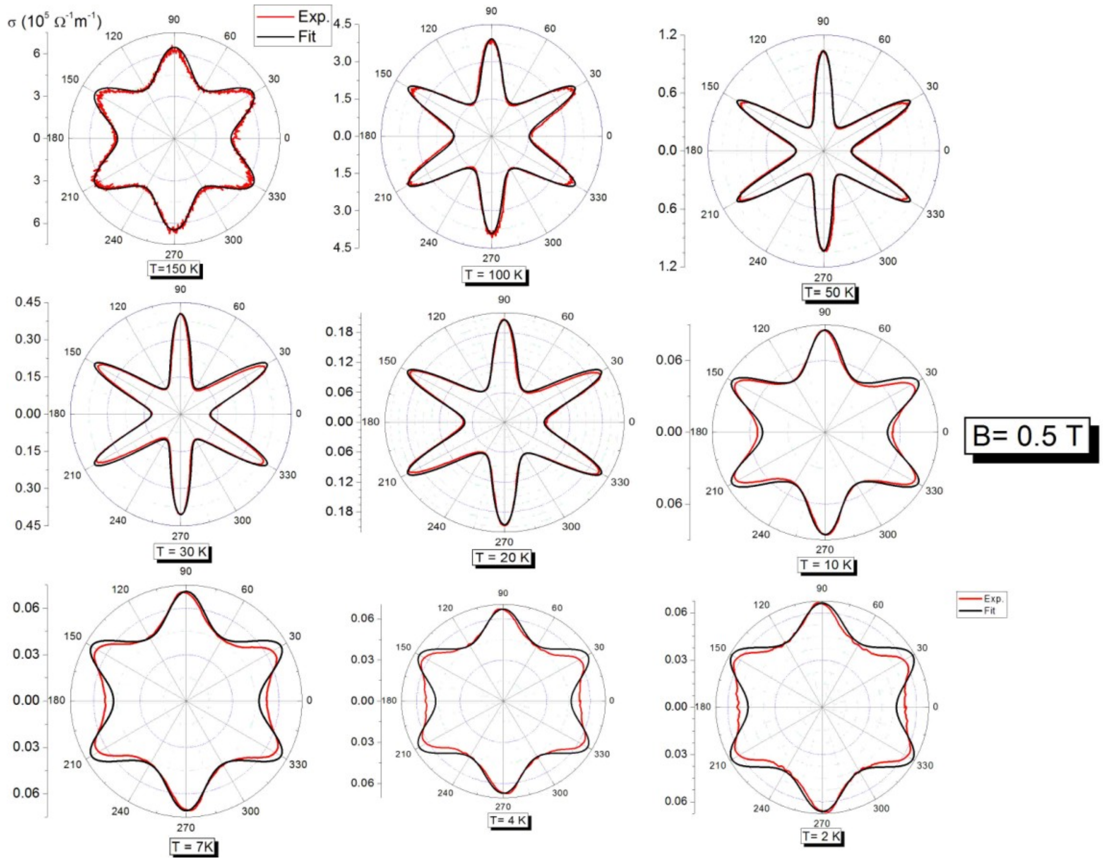


**FIG. S6** A comparison of experimental data of angle-dependent conductivity (red line) and the equation used to fit the data (black line). As seen in the data, the fit, which is quite successful at high temperature, fails below 10 K.

## REFERENCES


S1 J.-P. Issi, *Aust. J. Phys.* **32**, 585 (1979)

S2 R. Hartman, *Phys. Rev.* **181**, 1070 (1969)

S3 C. Uher and W. P. Pratt, Jr., *Phys. Rev. Lett.* **39**, 491 (1977)

S4 K. Anagnostopoulos and J. E. Aubrey, *J. Phys. F: Met. Phys.* **6** L181 (1976)

S5 S. Mase, S. von Molnar and A. W. Lawson, *Phys. Rev.* **127**, 1030 (1962)

S6 D. T. Morelli and C. Uher, *Phys. Rev. B* **30**, 1080 (1984)

S7 R. N. Zitter, *Phys. Rev.* **127**, 1471 (1962)
